# Supplementary material for: DISA: DIfferentiable Similarity Approximation for Universal Multimodal Registration
Source: arXiv:2307.09931 source file (2023-07-19)
Supplement: Supplementary file 1 [file appendix.tex]

\section{Comparison $LC^2$ vs DISA-$LC^2$}

\begin{figure}[h!]
\includegraphics[width=0.48\textwidth]{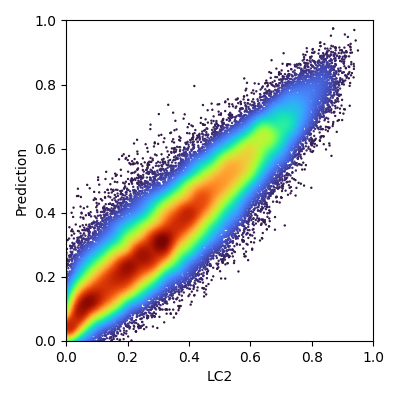}
\label{fig:heat_scatter}
\caption{Heat-scatterplot of the model prediction on the validation set}
\end{figure}

\section{Probe deformation model}
\commentMR{Here $\alpha$ is used again, should use a different letter}\\
We model the displacement due to the probe pressure as a spherical compression originating from a point $\vett{c}$ and acting from distance $r$ up to distance $R$. 
Our model has two parameters: $\alpha \in [0, 1]$ controls the intensity of the deformation, while $\beta \in [0, 10]$ controls the rate at which the deformation dissipates.
Concretely we formulate the displacement of a point $\vett{p}$ as follows:
$$
\vett{d}(\vett{p}, \alpha, \beta) = \alpha R \frac{\vett{p} - \vett{c}}{\norm{\vett{p} - \vett{c}}} f(\norm{\vett{p} - \vett{c}})^{1 + \beta}  \text{ where } f(x) = \begin{cases}
\frac{10x}{8r} & \text{if } x < \frac{8}{10}r \\
1 & \text{if } kr \leq x \leq r \\
1 - \frac{x - r}{R - r} & \text{if } r < x \leq R \\
0 & \text{if } x > R
\end{cases} \,.
$$
